# Supplementary material for: Improving Detail in Pluralistic Image Inpainting with Feature Dequantization
Source: arXiv:2412.01046 source file (2024-12-02)
Supplement: Supplementary file 1 [file appendix.tex]

\begin{table*}[hbt!]
  \caption{Comparison with deterministic inpainting model}
  \label{tab:deterministic}
  \centering
  {\small
  \begin{tabular}{@{\extracolsep{4pt}}p{0.15\textwidth}rrrrrrrr@{}}
    \toprule[1.2pt]
    \multirow{3}{*}{Methods} & \multicolumn{4}{c}{Places} & \multicolumn{4}{c}{Paris Street View} \\
    \cline{2-5} \cline{6-9}
    & \multicolumn{2}{c}{FID} & \multicolumn{2}{c}{LPIPS} & \multicolumn{2}{c}{FID} & \multicolumn{2}{c}{LPIPS} \\
    \cline{2-3} \cline{4-5} \cline{6-7} \cline{8-9}
    & small & large & small & large & small & large & small & large \\
    \hline
    % \df & 31.41 & 44.29 & 0.189 & 0.285 & \makecell[c]{-} & \makecell[c]{-} & \makecell[c]{-} & \makecell[c]{-} \\
    \lama & $\mathbf{17.30}$ & 29.86 & $\mathbf{0.120}$ & $\mathbf{0.213}$ & $\mathbf{10.89}$ & 21.79 & $\mathbf{0.124}$ & 0.236 \\
    % \cmt & 17.36 & 28.93 & 0.120 & 0.222 & \makecell[c]{-} & \makecell[c]{-} & \makecell[c]{-} & \makecell[c]{-}  \\
    \ourPUT & 18.46 & $\mathbf{29.67}$ & 0.127 & 0.230 & 11.63 & $\mathbf{18.66}$ & 0.131 & $\mathbf{0.234}$ \\
    \bottomrule[1.2pt]
  \end{tabular}}
\end{table*}

\begin{figure*}[hbt!]
  \centering
  \begin{subfigure}[t]{0.11\linewidth}
    \includegraphics[width=\textwidth]{figure/deterministic/places_gt3.jpg} \\
    \includegraphics[width=\textwidth]{figure/deterministic/paris_gt1.png}
    \caption*{GT}
  \end{subfigure} 
  \unskip\ \vrule\
  \begin{subfigure}[t]{0.11\linewidth}
    \includegraphics[width=\textwidth]{figure/deterministic/masks02_03/places_masked3.jpg} \\
    \includegraphics[width=\textwidth]{figure/deterministic/masks02_03/paris_masked1.png}
    \caption*{Input}
  \end{subfigure}
  \begin{subfigure}[t]{0.11\linewidth}
    \includegraphics[width=\textwidth]{figure/deterministic/masks02_03/places_lama3.jpg} \\
    \includegraphics[width=\textwidth]{figure/deterministic/masks02_03/paris_lama1.png}
    \caption*{LaMa}
  \end{subfigure}
  \begin{subfigure}[t]{0.11\linewidth}
    \includegraphics[width=\textwidth]{figure/deterministic/masks02_03/places_fdm3.jpg} \\
    \includegraphics[width=\textwidth]{figure/deterministic/masks02_03/paris_fdm1.png}
    \caption*{Ours}
  \end{subfigure}
  \unskip\ \vrule\
  \begin{subfigure}[t]{0.11\linewidth}
    \includegraphics[width=\textwidth]{figure/deterministic/masks05_06/places_masked3.jpg} \\
    \includegraphics[width=\textwidth]{figure/deterministic/masks05_06/paris_masked1.png}
    \caption*{Input}
  \end{subfigure}
  \begin{subfigure}[t]{0.11\linewidth}
    \includegraphics[width=\textwidth]{figure/deterministic/masks05_06/places_lama3.jpg} \\
    \includegraphics[width=\textwidth]{figure/deterministic/masks05_06/paris_lama1.png}
    \caption*{LaMa}
  \end{subfigure}
  \begin{subfigure}[t]{0.11\linewidth}
    \includegraphics[width=\textwidth]{figure/deterministic/masks05_06/places_fdm3.jpg} \\
    \includegraphics[width=\textwidth]{figure/deterministic/masks05_06/paris_fdm1.png}
    \caption*{Ours}
  \end{subfigure}
  \caption{Comparison with deterministic models across various mask ratios.}
  \label{fig:det_result}
\end{figure*}

\begin{table*}[hbt!]
  \caption{Quantitative results of different methods. \textbf{Bold} indicates the best score in PII methods.}
  \label{tab:main}
  \centering
  \resizebox{\textwidth}{!}{% 
  \begin{tabular}{@{\extracolsep{4pt}}p{0.10\textwidth}p{0.18\textwidth}rrrrrrrrrrrr@{}}
    \toprule[1.2pt]
    \multirow{3}{*}{Type} & Dataset & \multicolumn{6}{c}{Places \cite{zhou2017places}} & \multicolumn{6}{c}{Paris Street View \cite{doersch2012makes}} \\ \cline{3-8} \cline{9-14}
    & Metric & \multicolumn{2}{c}{MAE} & \multicolumn{2}{c}{SSIM} & \multicolumn{2}{c}{PSNR} & \multicolumn{2}{c}{MAE} & \multicolumn{2}{c}{SSIM} & \multicolumn{2}{c}{PSNR} \\
    \cline{3-4} \cline{5-6} \cline{7-8} \cline{9-10} \cline{11-12} \cline{13-14}
    & Mask Ratio  & small & large & small & large & small & large & small & large & small & large & small & large \\
    \hline
    DII & \lama & 0.024 & 0.045 & 0.868 & 0.707 & 26.19 & 22.38 & 0.025 & 0.053 & 0.897 & 0.764 & 25.94 & 21.94 \\
    \hline
    \multirow{4}{*}{PII} & \ict\cite{wan2021high} & 0.033 & 0.059 & 0.821 & 0.625 & 24.33 & 20.53 & 0.035 & 0.065 & 0.857 & 0.693 & 24.20 & 20.47 \\
    & \mat\cite{li2022mat} & 0.028 & $\mathbf{0.049}$ & $\mathbf{0.873}$ & $\mathbf{0.700}$ & $\mathbf{26.48}$ & $\mathbf{22.09}$ & 0.031 & 0.063 & 0.859 & 0.688 & 24.22 & 20.22 \\
    & \ldm\cite{rombach2022high} & $\mathbf{0.024}$ & 0.049 & 0.849 & 0.662 & 25.47 & 21.24 & 0.032 & 0.063 & 0.849 & 0.689 & 23.87 & 20.23 \\
    & \putModel\cite{liu2022reduce} & 0.028 & 0.054 & 0.840 & 0.649 & 25.07 & 20.88 & 0.031 & 0.059 & 0.875 & 0.729 & 24.90 & 21.11 \\
    & \ourPUT & 0.026 & 0.052 & 0.844 & 0.653 & 25.24 & 20.98 & $\mathbf{0.030}$ & $\mathbf{0.058}$ & $\mathbf{0.877}$ & $\mathbf{0.733}$ & $\mathbf{25.03}$ & $\mathbf{21.22}$ \\
    \bottomrule[1.2pt]
  \end{tabular}}
\end{table*}

\appendix

\section{Encoder-decoder Arcitecture}

In our proposed method, encoder-decoder has the same architecture as \putModel\cite{liu2022reduce}.

\minisection{Encoder}
The encoder is composed of 8 linear residual blocks and 2 linear layers.
Each block consists of a linear layer followed by a ReLU activation function.
After the linear layer, output is added to the input of the block and passed through a ReLU activation function.
In the encoding process, initially, the masked image $\defMaskedImg$ is transformed from RGB channels (3) to feature channels (256) through linear layers with ReLU activation functions.
Subsequently, the feature undergoes computation with linear residual blocks. 
Finally, to convert features channels into the codebook vector channels (256), it passes through a linear layer followed by a ReLU activation function.

\minisection{Decoder}
The decoder comprises two paths: a feature upsampling path and a masked image downsampling path.

The feature upsampling path consists of 8 convolutional residual blocks and 3 upsampling layers. Each block includes a $3\times3$ convolutional layer followed by a ReLU activation function and a $1\times1$ convolutional layer. Subsequently, the output of the $1\times1$ convolutional layer is added to the input of the block and passed through a ReLU activation function. Upsampling is conducted using $4\times4$ deconvolutional layers with a stride of 2.

The masked image downsampling path comprises 3 downsampling layers. Downsampling is executed using $3\times3$ convolutional layers followed by ReLU activation. In the feature upsampling path, features traverse through residual blocks before undergoing upsampling. Subsequently, the features are upsampled to match the image resolution. In the proposed method, the feature resolution is $32\times32$, and the image resolution is $256\times256$, thus 3 upsampling steps are performed.

At each upsampling step, the upsampled features are combined with the downsampled masked image using the following equation:

\begin{align}
\mathbf{f}_{n} = \mathbf{f}'_n \otimes (1-\mathbf{m}_n) + \hat{\mathbf{x}}_n \otimes \mathbf{m}_n
\end{align}

where $\mathbf{f}'_n$ represents the upsampled feature in the $n$-th step, $\hat{\mathbf{x}}_n$ denotes the downsampled masked image in the $n$-th step, and $\mathbf{m}_n$ signifies the downsampled mask in the $n$-th step.

Finally, to convert features channels (256) into the RGB channels (3), upsampled features passes through a $3\times3$ convolutional layer.

\section{Comparison with Deterministic Method}

% We compare the proposed method with the following state-of-the-art deterministic inpainting approaches: \df\cite{yu2019free} and \lama\cite{suvorov2022resolution}.
We compare the proposed method with the following state-of-the-art deterministic inpainting approach \lama\cite{suvorov2022resolution}.
Table~\ref{tab:deterministic} displays the quantitative results comparing our proposed approach, FDM, with \lama.
FDM shows competitive performance in terms of FID compared to the state-of-the-art model \lama.
Particularly, it demonstrates better performance, especially in the case of large masks.

Figure~\ref{fig:det_result} illustrates the inference results of FDM and Lama.
It can be observed that Lama's inpainting performance deteriorates when the mask ratio is high.
On the contrary, the proposed method generates natural images even as the mask ratio increases.

\lama sometimes fills the mask with a single color, as seen in the example when the mask ratio is wide.
In such cases, if the model generates unnatural images, users have no way to improve them.
In contrast, PII offers various generated results, thereby expanding the user's choice and increasing the likelihood of obtaining satisfactory results.

\section{Additional Quantitative Results}

Table~\ref{tab:main} presents a comparison of methods across MAE, PSNR and SSIM.
These metrics evaluate pixel-wise similarity between an output image and the ground-truth image, without considering diversity or alignment with human perception. 
Therefore, they are not suitable for evaluating pluralistic inpainting, as discussed in Section 4.1.

FDM converts quantized features into continuous features based on the predicted image structure by the feature sampler, without making them closer to the ground-truth features.
Therefore, FDM does not significantly improve the performance of \putModel\cite{liu2022reduce} in terms of PSNR, SSIM \cite{wang2004image}, and MAE, unlike in FID \cite{heusel2017gans} and LPIPS \cite{zhang2018unreasonable}.

As discussed in Section 4.4, the Paris Street View dataset \cite{doersch2012makes} contains a lot of noise, resulting in a decrease in both the performance improvement capability of FDM and the performance of \mat \cite{li2022mat} and \ldm\cite{rombach2022high}.
However, as discussed in Section 4.2, the proposed method demonstrates much greater diversity than MAT and achieves better FID scores than LDM with large masks.
Therefore, our proposed method has been proven to generate diverse and natural-looking images.

\section{Additional Qualitative Results}

Figure~\ref{fig:sup_detail_inp_result} provides a more detail comparison between \putModel\cite{liu2022reduce} and our proposed method.
\putModel produce color discrepancies and distorted structures or fails to properly represent texture.
For example, in row 1 and 3, \putModel generates the window grilles inconsistently or unclearly.
However, our proposed method generates the window grilles in a straight line without interruption.

Figure~\ref{fig:sup_div_inp_result_places} and Figure~\ref{fig:sup_div_inp_result_paris} provide more visual comparison of diverse inpainting results among PII methods.
In \ict\cite{wan2021high} and \ldm\cite{rombach2022high}, artifacts have been generated, such as blurring or structural ambiguity.
Although \mat\cite{li2022mat} shows few artifacts, it often generates structurally similar images, resulting in limited diversity in the results.
In contrast, our proposed method has successfully generated diverse images while preserving naturalness.

\begin{figure*}[tb]
  \centering
  \begin{subfigure}[t]{0.2\linewidth}
    \includegraphics[width=\textwidth]{figure/appendix/detail/paris_1_masked.jpg} \\
    \includegraphics[width=\textwidth]{figure/appendix/detail/paris_2_masked.jpg} \\
    \includegraphics[width=\textwidth]{figure/appendix/detail/paris_3_masked.jpg} \\
    \includegraphics[width=\textwidth]{figure/appendix/detail/places2_6_masked.jpg} \\
    \includegraphics[width=\textwidth]{figure/appendix/detail/places2_3_masked.jpg} \\
    \includegraphics[width=\textwidth]{figure/appendix/detail/places2_4_masked.jpg} \\
    \caption*{Input}
  \end{subfigure}
  \begin{subfigure}[t]{0.2\linewidth}
    \includegraphics[width=\textwidth]{figure/appendix/detail/paris_1_PUT.jpg} \\
    \includegraphics[width=\textwidth]{figure/appendix/detail/paris_2_PUT.jpg} \\
    \includegraphics[width=\textwidth]{figure/appendix/detail/paris_3_PUT.jpg} \\
    \includegraphics[width=\textwidth]{figure/appendix/detail/places2_6_PUT.jpg} \\
    \includegraphics[width=\textwidth]{figure/appendix/detail/places2_3_PUT.jpg} \\
    \includegraphics[width=\textwidth]{figure/appendix/detail/places2_4_PUT.jpg} \\
    \caption*{PUT}
  \end{subfigure}
  \begin{subfigure}[t]{0.2\linewidth}
    \includegraphics[width=\textwidth]{figure/appendix/detail/paris_1_FDM.jpg} \\
    \includegraphics[width=\textwidth]{figure/appendix/detail/paris_2_FDM.jpg} \\
    \includegraphics[width=\textwidth]{figure/appendix/detail/paris_3_FDM.jpg} \\
    \includegraphics[width=\textwidth]{figure/appendix/detail/places2_6_FDM.jpg} \\
    \includegraphics[width=\textwidth]{figure/appendix/detail/places2_3_FDM.jpg} \\
    \includegraphics[width=\textwidth]{figure/appendix/detail/places2_4_FDM.jpg} \\
    \caption*{Ours}
  \end{subfigure}
  \caption{Detail comparison between proposed method and PUT.}
  \label{fig:sup_detail_inp_result}
\end{figure*}

\begin{figure*}[tb]
  \centering
  \begin{subfigure}[t]{0.12\linewidth}
    \includegraphics[width=\textwidth]{figure/appendix/diversity/places_1_GT.jpg}
    \caption*{GT}
  \end{subfigure}
  \begin{subfigure}[t]{0.12\linewidth}
    \includegraphics[width=\textwidth]{figure/appendix/diversity/places_1_ICT1.jpg}
    \caption*{ICT1}
  \end{subfigure}
  \begin{subfigure}[t]{0.12\linewidth}
    \includegraphics[width=\textwidth]{figure/appendix/diversity/places_1_ICT2.jpg}
    \caption*{ICT2}
  \end{subfigure}
  \begin{subfigure}[t]{0.12\linewidth}
    \includegraphics[width=\textwidth]{figure/appendix/diversity/places_1_ICT3.jpg}
    \caption*{ICT3}
  \end{subfigure}
  \begin{subfigure}[t]{0.12\linewidth}
    \includegraphics[width=\textwidth]{figure/appendix/diversity/places_1_LDM1.png}
    \caption*{LDM1}
  \end{subfigure}
  \begin{subfigure}[t]{0.12\linewidth}
    \includegraphics[width=\textwidth]{figure/appendix/diversity/places_1_LDM2.png}
    \caption*{LDM2}
  \end{subfigure}
  \begin{subfigure}[t]{0.12\linewidth}
    \includegraphics[width=\textwidth]{figure/appendix/diversity/places_1_LDM3.png}
    \caption*{LDM3}
  \end{subfigure}
  
  \smallskip
  \begin{subfigure}[t]{0.12\linewidth}
    \includegraphics[width=\textwidth]{figure/appendix/diversity/places_1_masked.jpg}
    \caption*{Input}
  \end{subfigure}
  \begin{subfigure}[t]{0.12\linewidth}
    \includegraphics[width=\textwidth]{figure/appendix/diversity/places_1_MAT1.jpg}
    \caption*{MAT1}
  \end{subfigure}
  \begin{subfigure}[t]{0.12\linewidth}
    \includegraphics[width=\textwidth]{figure/appendix/diversity/places_1_MAT2.jpg}
    \caption*{MAT2}
  \end{subfigure}
  \begin{subfigure}[t]{0.12\linewidth}
    \includegraphics[width=\textwidth]{figure/appendix/diversity/places_1_MAT3.jpg}
    \caption*{MAT3}
  \end{subfigure}
  \begin{subfigure}[t]{0.12\linewidth}
    \includegraphics[width=\textwidth]{figure/appendix/diversity/places_1_FDM1.jpg}
    \caption*{Ours1}
  \end{subfigure}
  \begin{subfigure}[t]{0.12\linewidth}
    \includegraphics[width=\textwidth]{figure/appendix/diversity/places_1_FDM3.jpg}
    \caption*{Ours2}
  \end{subfigure}
  \begin{subfigure}[t]{0.12\linewidth}
    \includegraphics[width=\textwidth]{figure/appendix/diversity/places_1_FDM4.jpg}
    \caption*{Ours3}
  \end{subfigure}

  \bigskip
  \begin{subfigure}[t]{0.12\linewidth}
    \includegraphics[width=\textwidth]{figure/appendix/diversity/places_2_GT.jpg}
    \caption*{GT}
  \end{subfigure}
  \begin{subfigure}[t]{0.12\linewidth}
    \includegraphics[width=\textwidth]{figure/appendix/diversity/places_2_ICT1.jpg}
    \caption*{ICT1}
  \end{subfigure}
  \begin{subfigure}[t]{0.12\linewidth}
    \includegraphics[width=\textwidth]{figure/appendix/diversity/places_2_ICT2.jpg}
    \caption*{ICT2}
  \end{subfigure}
  \begin{subfigure}[t]{0.12\linewidth}
    \includegraphics[width=\textwidth]{figure/appendix/diversity/places_2_ICT3.jpg}
    \caption*{ICT3}
  \end{subfigure}
  \begin{subfigure}[t]{0.12\linewidth}
    \includegraphics[width=\textwidth]{figure/appendix/diversity/places_2_LDM1.png}
    \caption*{LDM1}
  \end{subfigure}
  \begin{subfigure}[t]{0.12\linewidth}
    \includegraphics[width=\textwidth]{figure/appendix/diversity/places_2_LDM2.png}
    \caption*{LDM2}
  \end{subfigure}
  \begin{subfigure}[t]{0.12\linewidth}
    \includegraphics[width=\textwidth]{figure/appendix/diversity/places_2_LDM3.png}
    \caption*{LDM3}
  \end{subfigure}
  
  \smallskip
  \begin{subfigure}[t]{0.12\linewidth}
    \includegraphics[width=\textwidth]{figure/appendix/diversity/places_2_masked.jpg}
    \caption*{Input}
  \end{subfigure}
  \begin{subfigure}[t]{0.12\linewidth}
    \includegraphics[width=\textwidth]{figure/appendix/diversity/places_2_MAT1.jpg}
    \caption*{MAT1}
  \end{subfigure}
  \begin{subfigure}[t]{0.12\linewidth}
    \includegraphics[width=\textwidth]{figure/appendix/diversity/places_2_MAT2.jpg}
    \caption*{MAT2}
  \end{subfigure}
  \begin{subfigure}[t]{0.12\linewidth}
    \includegraphics[width=\textwidth]{figure/appendix/diversity/places_2_MAT3.jpg}
    \caption*{MAT3}
  \end{subfigure}
  \begin{subfigure}[t]{0.12\linewidth}
    \includegraphics[width=\textwidth]{figure/appendix/diversity/places_2_FDM1.jpg}
    \caption*{Ours1}
  \end{subfigure}
  \begin{subfigure}[t]{0.12\linewidth}
    \includegraphics[width=\textwidth]{figure/appendix/diversity/places_2_FDM3.jpg}
    \caption*{Ours2}
  \end{subfigure}
  \begin{subfigure}[t]{0.12\linewidth}
    \includegraphics[width=\textwidth]{figure/appendix/diversity/places_2_FDM4.jpg}
    \caption*{Ours3}
  \end{subfigure}

  \bigskip
  \begin{subfigure}[t]{0.12\linewidth}
    \includegraphics[width=\textwidth]{figure/appendix/diversity/places_3_GT.jpg}
    \caption*{GT}
  \end{subfigure}
  \begin{subfigure}[t]{0.12\linewidth}
    \includegraphics[width=\textwidth]{figure/appendix/diversity/places_3_ICT1.jpg}
    \caption*{ICT1}
  \end{subfigure}
  \begin{subfigure}[t]{0.12\linewidth}
    \includegraphics[width=\textwidth]{figure/appendix/diversity/places_3_ICT2.jpg}
    \caption*{ICT2}
  \end{subfigure}
  \begin{subfigure}[t]{0.12\linewidth}
    \includegraphics[width=\textwidth]{figure/appendix/diversity/places_3_ICT3.jpg}
    \caption*{ICT3}
  \end{subfigure}
  \begin{subfigure}[t]{0.12\linewidth}
    \includegraphics[width=\textwidth]{figure/appendix/diversity/places_3_LDM1.png}
    \caption*{LDM1}
  \end{subfigure}
  \begin{subfigure}[t]{0.12\linewidth}
    \includegraphics[width=\textwidth]{figure/appendix/diversity/places_3_LDM2.png}
    \caption*{LDM2}
  \end{subfigure}
  \begin{subfigure}[t]{0.12\linewidth}
    \includegraphics[width=\textwidth]{figure/appendix/diversity/places_3_LDM3.png}
    \caption*{LDM3}
  \end{subfigure}
  
  \smallskip
  \begin{subfigure}[t]{0.12\linewidth}
    \includegraphics[width=\textwidth]{figure/appendix/diversity/places_3_masked.jpg}
    \caption*{Input}
  \end{subfigure}
  \begin{subfigure}[t]{0.12\linewidth}
    \includegraphics[width=\textwidth]{figure/appendix/diversity/places_3_MAT1.jpg}
    \caption*{MAT1}
  \end{subfigure}
  \begin{subfigure}[t]{0.12\linewidth}
    \includegraphics[width=\textwidth]{figure/appendix/diversity/places_3_MAT2.jpg}
    \caption*{MAT2}
  \end{subfigure}
  \begin{subfigure}[t]{0.12\linewidth}
    \includegraphics[width=\textwidth]{figure/appendix/diversity/places_3_MAT3.jpg}
    \caption*{MAT3}
  \end{subfigure}
  \begin{subfigure}[t]{0.12\linewidth}
    \includegraphics[width=\textwidth]{figure/appendix/diversity/places_3_FDM1.jpg}
    \caption*{Ours1}
  \end{subfigure}
  \begin{subfigure}[t]{0.12\linewidth}
    \includegraphics[width=\textwidth]{figure/appendix/diversity/places_3_FDM3.jpg}
    \caption*{Ours2}
  \end{subfigure}
  \begin{subfigure}[t]{0.12\linewidth}
    \includegraphics[width=\textwidth]{figure/appendix/diversity/places_3_FDM4.jpg}
    \caption*{Ours3}
  \end{subfigure}
  \caption{Visual comparison of diverse inpainting results in Places}
  \label{fig:sup_div_inp_result_places}
\end{figure*}

\begin{figure*}[tb]
  \centering
  \begin{subfigure}[t]{0.12\linewidth}
    \includegraphics[width=\textwidth]{figure/appendix/diversity/paris_1_GT.png}
    \caption*{GT}
  \end{subfigure}
  \begin{subfigure}[t]{0.12\linewidth}
    \includegraphics[width=\textwidth]{figure/appendix/diversity/paris_1_ICT1.png}
    \caption*{ICT1}
  \end{subfigure}
  \begin{subfigure}[t]{0.12\linewidth}
    \includegraphics[width=\textwidth]{figure/appendix/diversity/paris_1_ICT2.png}
    \caption*{ICT2}
  \end{subfigure}
  \begin{subfigure}[t]{0.12\linewidth}
    \includegraphics[width=\textwidth]{figure/appendix/diversity/paris_1_ICT3.png}
    \caption*{ICT3}
  \end{subfigure}
  \begin{subfigure}[t]{0.12\linewidth}
    \includegraphics[width=\textwidth]{figure/appendix/diversity/paris_1_LDM1.png}
    \caption*{LDM1}
  \end{subfigure}
  \begin{subfigure}[t]{0.12\linewidth}
    \includegraphics[width=\textwidth]{figure/appendix/diversity/paris_1_LDM2.png}
    \caption*{LDM2}
  \end{subfigure}
  \begin{subfigure}[t]{0.12\linewidth}
    \includegraphics[width=\textwidth]{figure/appendix/diversity/paris_1_LDM3.png}
    \caption*{LDM3}
  \end{subfigure}
  
  \smallskip
  \begin{subfigure}[t]{0.12\linewidth}
    \includegraphics[width=\textwidth]{figure/appendix/diversity/paris_1_masked.png}
    \caption*{Input}
  \end{subfigure}
  \begin{subfigure}[t]{0.12\linewidth}
    \includegraphics[width=\textwidth]{figure/appendix/diversity/paris_1_MAT1.png}
    \caption*{MAT1}
  \end{subfigure}
  \begin{subfigure}[t]{0.12\linewidth}
    \includegraphics[width=\textwidth]{figure/appendix/diversity/paris_1_MAT2.png}
    \caption*{MAT2}
  \end{subfigure}
  \begin{subfigure}[t]{0.12\linewidth}
    \includegraphics[width=\textwidth]{figure/appendix/diversity/paris_1_MAT3.png}
    \caption*{MAT3}
  \end{subfigure}
  \begin{subfigure}[t]{0.12\linewidth}
    \includegraphics[width=\textwidth]{figure/appendix/diversity/paris_1_FDM1.png}
    \caption*{Ours1}
  \end{subfigure}
  \begin{subfigure}[t]{0.12\linewidth}
    \includegraphics[width=\textwidth]{figure/appendix/diversity/paris_1_FDM3.png}
    \caption*{Ours2}
  \end{subfigure}
  \begin{subfigure}[t]{0.12\linewidth}
    \includegraphics[width=\textwidth]{figure/appendix/diversity/paris_1_FDM4.png}
    \caption*{Ours3}
  \end{subfigure}

  \bigskip
  \begin{subfigure}[t]{0.12\linewidth}
    \includegraphics[width=\textwidth]{figure/appendix/diversity/paris_2_GT.png}
    \caption*{GT}
  \end{subfigure}
  \begin{subfigure}[t]{0.12\linewidth}
    \includegraphics[width=\textwidth]{figure/appendix/diversity/paris_2_ICT1.png}
    \caption*{ICT1}
  \end{subfigure}
  \begin{subfigure}[t]{0.12\linewidth}
    \includegraphics[width=\textwidth]{figure/appendix/diversity/paris_2_ICT2.png}
    \caption*{ICT2}
  \end{subfigure}
  \begin{subfigure}[t]{0.12\linewidth}
    \includegraphics[width=\textwidth]{figure/appendix/diversity/paris_2_ICT3.png}
    \caption*{ICT3}
  \end{subfigure}
  \begin{subfigure}[t]{0.12\linewidth}
    \includegraphics[width=\textwidth]{figure/appendix/diversity/paris_2_LDM1.png}
    \caption*{LDM1}
  \end{subfigure}
  \begin{subfigure}[t]{0.12\linewidth}
    \includegraphics[width=\textwidth]{figure/appendix/diversity/paris_2_LDM2.png}
    \caption*{LDM2}
  \end{subfigure}
  \begin{subfigure}[t]{0.12\linewidth}
    \includegraphics[width=\textwidth]{figure/appendix/diversity/paris_2_LDM3.png}
    \caption*{LDM3}
  \end{subfigure}
  
  \smallskip
  \begin{subfigure}[t]{0.12\linewidth}
    \includegraphics[width=\textwidth]{figure/appendix/diversity/paris_2_masked.png}
    \caption*{Input}
  \end{subfigure}
  \begin{subfigure}[t]{0.12\linewidth}
    \includegraphics[width=\textwidth]{figure/appendix/diversity/paris_2_MAT1.png}
    \caption*{MAT1}
  \end{subfigure}
  \begin{subfigure}[t]{0.12\linewidth}
    \includegraphics[width=\textwidth]{figure/appendix/diversity/paris_2_MAT2.png}
    \caption*{MAT2}
  \end{subfigure}
  \begin{subfigure}[t]{0.12\linewidth}
    \includegraphics[width=\textwidth]{figure/appendix/diversity/paris_2_MAT3.png}
    \caption*{MAT3}
  \end{subfigure}
  \begin{subfigure}[t]{0.12\linewidth}
    \includegraphics[width=\textwidth]{figure/appendix/diversity/paris_2_FDM1.png}
    \caption*{Ours1}
  \end{subfigure}
  \begin{subfigure}[t]{0.12\linewidth}
    \includegraphics[width=\textwidth]{figure/appendix/diversity/paris_2_FDM3.png}
    \caption*{Ours2}
  \end{subfigure}
  \begin{subfigure}[t]{0.12\linewidth}
    \includegraphics[width=\textwidth]{figure/appendix/diversity/paris_2_FDM4.png}
    \caption*{Ours3}
  \end{subfigure}

  \bigskip
  \begin{subfigure}[t]{0.12\linewidth}
    \includegraphics[width=\textwidth]{figure/appendix/diversity/paris_3_GT.png}
    \caption*{GT}
  \end{subfigure}
  \begin{subfigure}[t]{0.12\linewidth}
    \includegraphics[width=\textwidth]{figure/appendix/diversity/paris_3_ICT1.png}
    \caption*{ICT1}
  \end{subfigure}
  \begin{subfigure}[t]{0.12\linewidth}
    \includegraphics[width=\textwidth]{figure/appendix/diversity/paris_3_ICT2.png}
    \caption*{ICT2}
  \end{subfigure}
  \begin{subfigure}[t]{0.12\linewidth}
    \includegraphics[width=\textwidth]{figure/appendix/diversity/paris_3_ICT3.png}
    \caption*{ICT3}
  \end{subfigure}
  \begin{subfigure}[t]{0.12\linewidth}
    \includegraphics[width=\textwidth]{figure/appendix/diversity/paris_3_LDM1.png}
    \caption*{LDM1}
  \end{subfigure}
  \begin{subfigure}[t]{0.12\linewidth}
    \includegraphics[width=\textwidth]{figure/appendix/diversity/paris_3_LDM2.png}
    \caption*{LDM2}
  \end{subfigure}
  \begin{subfigure}[t]{0.12\linewidth}
    \includegraphics[width=\textwidth]{figure/appendix/diversity/paris_3_LDM3.png}
    \caption*{LDM3}
  \end{subfigure}
  
  \smallskip
  \begin{subfigure}[t]{0.12\linewidth}
    \includegraphics[width=\textwidth]{figure/appendix/diversity/paris_3_masked.png}
    \caption*{Input}
  \end{subfigure}
  \begin{subfigure}[t]{0.12\linewidth}
    \includegraphics[width=\textwidth]{figure/appendix/diversity/paris_3_MAT1.png}
    \caption*{MAT1}
  \end{subfigure}
  \begin{subfigure}[t]{0.12\linewidth}
    \includegraphics[width=\textwidth]{figure/appendix/diversity/paris_3_MAT2.png}
    \caption*{MAT2}
  \end{subfigure}
  \begin{subfigure}[t]{0.12\linewidth}
    \includegraphics[width=\textwidth]{figure/appendix/diversity/paris_3_MAT3.png}
    \caption*{MAT3}
  \end{subfigure}
  \begin{subfigure}[t]{0.12\linewidth}
    \includegraphics[width=\textwidth]{figure/appendix/diversity/paris_3_FDM1.png}
    \caption*{Ours1}
  \end{subfigure}
  \begin{subfigure}[t]{0.12\linewidth}
    \includegraphics[width=\textwidth]{figure/appendix/diversity/paris_3_FDM3.png}
    \caption*{Ours2}
  \end{subfigure}
  \begin{subfigure}[t]{0.12\linewidth}
    \includegraphics[width=\textwidth]{figure/appendix/diversity/paris_3_FDM4.png}
    \caption*{Ours3}
  \end{subfigure}
  \caption{Visual comparison of diverse inpainting results in Paris Street View}
  \label{fig:sup_div_inp_result_paris}
\end{figure*}
